# Supplementary material for: VibeVideoBench: Evaluating Multimodal Agents on Code-Driven Video Generation
Source: arXiv:2610.35864 source file (2026-12-01)
Supplement: Supplementary file 1 [file full_rows_239.tex]

1 & \lab{labOAI}GPT-6 Astra & Codex CLI & 8.19 & \second{99.6} & 93.7 & \second{97.1} & \best{4.08} & \best{4.30} & \best{4.20} & \best{3.95} & \best{4.10} & \cellcolor{best}\textbf{4.126} & \second{96.9} & \second{74.5} & \best{4.109}\,{\scriptsize\textcolor{black!45}{(1)}} & \best{1242} \\
2 & \lab{labANT}Claude Opus 5.5 & Claude Code & 15.38 & \best{100.0} & \best{99.6} & \best{97.3} & \second{3.99} & \second{4.19} & \second{4.18} & \best{3.95} & 4.07 & \second{4.074} & \best{97.3} & \best{76.3} & \second{4.074}\,{\scriptsize\textcolor{black!45}{(2)}} & \second{1203} \\
3 & \lab{labANT}Claude Sonnet 5.5 & Claude Code & 8.26 & 97.1 & \second{94.6} & 93.9 & 3.93 & 4.12 & 4.10 & \second{3.86} & 3.98 & 3.999 & 91.2 & 66.9 & 3.880\,{\scriptsize\textcolor{black!45}{(4)}} & 1121 \\
4 & \lab{labGOO}Gemini 4 Argon & Antigravity CLI & 2.94 & 77.0 & 76.6 & 96.5 & 3.80 & 4.05 & 4.14 & \second{3.86} & \second{4.09} & 3.989 & 73.5 & 55.2 & 3.069\,{\scriptsize\textcolor{black!45}{(7)}} & 1081 \\
5 & \lab{labDS}DeepSeek-V4.1-Flash & DSH & 0.47 & 98.7 & \second{94.6} & 93.1 & 3.86 & 4.13 & 4.04 & 3.75 & 4.03 & 3.961 & 92.0 & 57.6 & 3.911\,{\scriptsize\textcolor{black!45}{(3)}} & 1022 \\
6 & \lab{labMS}Kimi K3 & Kimi Code & 3.53 & 89.1 & 85.8 & 91.1 & 3.73 & 3.98 & 3.97 & 3.70 & 3.95 & 3.864 & 79.3 & 46.3 & 3.440\,{\scriptsize\textcolor{black!45}{(5)}} & 997 \\
7 & \lab{labZP}GLM-5.3-Flash & ZCode & 0.32 & 74.9 & 66.9 & 85.3 & 3.66 & 3.87 & 3.77 & 3.57 & 3.81 & 3.736 & 61.7 & 33.5 & 2.790\,{\scriptsize\textcolor{black!45}{(9)}} & 905 \\
8 & \lab{labOAI}GPT-5.6 Sol & Codex CLI & 11.84 & 89.1 & 84.5 & 89.5 & 3.72 & 3.94 & 3.86 & 3.45 & 3.71 & 3.735 & 78.0 & 39.1 & 3.317\,{\scriptsize\textcolor{black!45}{(6)}} & 705 \\
9 & \lab{labGOO}Gemini 3.8 Flash & Antigravity CLI & 2.44 & 80.8 & 77.4 & 80.4 & 3.33 & 3.57 & 3.59 & 3.12 & 3.74 & 3.470 & 61.3 & 26.6 & 2.798\,{\scriptsize\textcolor{black!45}{(8)}} & 723 \\
